# Supplementary material for: Articulation in Motion: Prior-free Part Mobility Analysis for Articulated Objects By Dynamic-Static Disentanglement
Source: arXiv:2603.02910 source file (2026-03-03)
Supplement: Supplementary file 1 [file supp.tex]

\begin{table}[t]
\centering
    \begin{minipage}[b]{0.45\linewidth}
    \centering
        \caption{}
        \vspace{-2mm}
        \resizebox{0.9\textwidth}{!}{ 
    \begin{tabular}{c|c|c|c|c|c}
    \toprule
    & 3D IoU & PARIS-m & DTA & ArtGS & Ours\\
    \midrule
    & $S$ &\multirow{4}*{F} & 90.55$_{\pm2.54}$ &91.84$_{\pm7.51}$&\\
    Storage& $D_0$ & & 24.38$_{\pm 5.41}$ & 51.80$_{\pm47.16}$ &\\
    \textit{47024}& $D_1$ & & 35.37$_{\pm35.35}$ & 94.89$_{\pm2.32}$  &\\
    & Mean & & 50.10$_{\pm14.01}$ & 79.51$_{\pm18.96}$ &\\
    \midrule
    &$S$ & & 81.05$_{\pm4.28}$ & 94.86$_{\pm0.61}$&\\
    Fridge&$D_0$ & & 33.84$_{\pm27.12}$ &  85.46$_{\pm2.37}$ &\\
    \textit{11304}&  $D_1$ & & 16.19$_{\pm21.48}$ &  66.24$_{\pm16.73}$&\\
    & Mean & & 43.69$_{\pm16.11}$ & 85.46$_{\pm6.29}$ &\\
      \bottomrule
    \end{tabular}}
        % \vspace{-2.5mm}
        \label{tab:ablation_scan_overall}
    \end{minipage}
    \hspace{5mm}
    \begin{minipage}[b]{0.45\linewidth}
    \centering
        \caption{Ablation on \textbf{the scanning directions} on the Matterport dataset.}
        \vspace{-2mm}
        \resizebox{1\textwidth}{!}{ 
    \begin{tabular}{c|c|c|c|c}
    \toprule
    &3D IoU ($\%$) & DTA & ArtGS & Ours\\
    \midrule
     \multirow{3}*{\textit{$\text{Storage}_{\text{47648}}$}}& $S$ & \multirow{3}*{F}  & &\\
    & $D_{avg}$ && &\\
    & Mean &  & &\\
    \midrule
    \multirow{3}*{\textit{$\text{Table}_{\text{31249}}$}}& $S$ & 87.95$_{\pm1.82}$& &\\
    & $D_{avg}$ &11.52$_{\pm10.96}$  & &\\
    & Mean & 26.81$_{\pm8.71}$ & & \\
      \bottomrule
    \end{tabular}}
    \label{tab:ablation_scan_overall}
    \end{minipage}
\end{table}
\begin{table}[t]
    \caption{\textbf{Quantitative evaluation of part segmentation on two-part objects.} 
Results are reported over 10 trials as mean$\pm$std. 
Ours-b fails on \textit{washer} and PARIS fails on \textit{stapler} and \textit{USB}, denoted as $F$. 
Higher IoU ($\uparrow$) indicates better performance, and \tblue{best} results are highlighted. \underline{Underline} shows the results are comparative.
}
    \vspace{-5pt}
    \label{tab:comparison-ps1}
    \resizebox{1\textwidth}{!}{ 
    \begin{tabular}{c|c|c|c|c|c|c|c|c}
    \toprule
    \multirow{2}*{3D IoU (\%) $\uparrow$} & \multirow{2}*{Method}& \multicolumn{7}{c}{Two-part objects}\\
    \cmidrule{3-9}
    & &Fridge& Oven& Scissor& USB& Washer& Blade& Storage\\
    \midrule
        \rowcolor{gray!20}
     \cellcolor{white}& PARIS& 85.23$_{\pm9.20}$  & 92.19$_{\pm6.33}$ &83.13$_{\pm3.71}$& F&\underline{98.53$_{\pm0.48}$}&\underline{87.84$_{\pm2.60}$}& 86.73$_{\pm3.18}$\\
        \rowcolor{gray!20}
     \cellcolor{white}Static& DTA& 86.27$_{\pm6.58}$  & 91.11$_{\pm3.50}$ &66.01$_{\pm3.38}$ &86.30$_{\pm1.84}$&88.49$_{\pm10.94}$ & 83.22$_{\pm2.03}$ & 88.87$_{\pm1.84}$ \\
    \rowcolor{gray!20}
     \cellcolor{white}Part& ArtGS& 87.69$_{\pm10.46}$  & 94.55$_{\pm3.76}$ &84.70$_{\pm4.27}$&   88.62$_{\pm2.32}$ &94.51$_{\pm4.04}$&90.91$_{\pm1.57}$&88.68$_{\pm2.66}$ \\

    \cellcolor{white}& Ours-b & 83.70$_{\pm4.70}$  & 94.46$_{\pm2.31}$ &81.27$_{\pm2.84}$&  55.15$_{\pm14.96}$& F & 83.59$_{\pm1.41}$& 88.57$_{\pm 3.07}$\\
    \cellcolor{white}& Ours& \tblue{88.01$_{\pm6.37}$}  & \tblue{97.72$_{\pm0.52}$} &\tblue{92.42$_{\pm1.05}$}& \tblue{92.93$_{\pm1.30}$}& \underline{96.98$_{\pm2.22}$}& \underline{84.33$_{\pm1.65}$} & \tblue{91.41$_{\pm2.78}$}\\
    \midrule
    \rowcolor{gray!20}
    \cellcolor{white}&PARIS& 55.97$_{\pm29.62}$  &45.42$_{\pm43.90}$ &67.81$_{\pm 15.09}$& F&32.75$_{\pm29.62}$&34.42$_{\pm10.85}$ & 42.88$_{\pm16.99}$\\
    \rowcolor{gray!20}
    \cellcolor{white}Dynamic& DTA& 52.06$_{\pm22.22}$  &41.23$_{\pm22.06}$ &53.58$_{\pm7.44}$&79.81$_{\pm2.71}$&5.97$_{\pm5.64}$&27.92$_{\pm11.62}$&39.01$_{\pm10.74}$\\
    \rowcolor{gray!20}
    \cellcolor{white}Part& ArtGS& 58.78$_{\pm36.40}$  & 65.68$_{\pm24.50}$ &75.04$_{\pm9.69}$&86.85$_{\pm2.37}$& 35.62$_{\pm36.43}$&28.95$_{\pm16.08}$ &65.30$_{\pm9.66}$ \\

     \cellcolor{white}& Ours-b& 57.09$_{\pm17.60}$  &72.50$_{\pm9.45}$ &77.74$_{\pm 3.75}$ & 55.36$_{\pm14.52}$& F&41.76$_{\pm3.34}$ & 35.54$_{\pm 26.04}$\\

    \cellcolor{white}& Ours& \tblue{75.19$_{\pm14.61}$}  &\tblue{89.61$_{\pm1.50}$} &\tblue{92.21$_{\pm 1.19}$}& \tblue{91.95$_{\pm1.18}$}& \tblue{68.52$_{\pm13.80}$}& \tblue{43.92$_{\pm6.97}$} & \tblue{69.01$_{\pm7.42}$} \\
    \midrule
          \rowcolor{gray!20}
    \cellcolor{white}&PARIS& 70.60$_{\pm19.40}$ & 68.80$_{\pm25.11}$ & 75.47$_{\pm 9.01}$& F &65.64$_{\pm14.34}$ &61.13$_{\pm6.64}$&64.81$_{\pm10.08}$\\
          \rowcolor{gray!20}
    \cellcolor{white}& DTA& 69.16$_{\pm13.56}$ & 66.17$_{\pm12.75}$ & 59.79$_{\pm 5.41}$ &83.05$_{\pm2.26}$&47.23$_{\pm6.89}$&55.57$_{\pm6.80}$ &63.94$_{\pm4.57}$\\
      \rowcolor{gray!20}
    \cellcolor{white}Mean& ArtGS&  73.24$_{\pm23.42}$  & 80.12$_{\pm14.13}$ &79.87$_{\pm6.19}$& 87.73$_{\pm2.10}$& 65.06$_{\pm20.21}$&59.93$_{\pm8.82}$ &76.99$_{\pm6.17}$\\

     \cellcolor{white}& Ours-b& 70.40$_{\pm11.13}$ & 83.48$_{\pm5.86}$ & 79.51$_{\pm 3.26}$&  55.26$_{\pm14.51}$& F & 62.68$_{\pm2.47}$  & 62.06$_{\pm 13.79}$\\

    \cellcolor{white}& Ours& \tblue{81.60$_{\pm10.48}$} & \tblue{93.66$_{\pm0.98}$} & \tblue{92.31$_{\pm 1.12}$}& \tblue{92.44$_{\pm1.24}$}& \tblue{82.75$_{\pm7.99}$ }&\tblue{64.12$_{\pm4.29}$} & \tblue{80.21$_{\pm7.37}$}\\
      \bottomrule
    \end{tabular}}
    \vspace{-5pt}
\end{table}
\begin{table}[t]
\centering
\vspace{-5pt}
    \begin{minipage}[b]{0.45\linewidth}
    \centering
        \caption{\textbf{Performance on three-part objects.} we report mean values of 3D IoU ($\%$) across 10 trials. }
        \vspace{-2mm}
        \resizebox{1\textwidth}{!}{ 
    \begin{tabular}{c|c|c|c|c|c}
    \toprule
    & 3D IoU & PARIS-m & DTA & ArtGS & Ours\\
    \midrule
    & $S$ & 89.77 & 88.53 &92.23& \tblue{94.20}\\
    Storage& $D_0$ & \multirow{2}*{F} & 55.32 & 51.78 & \tblue{94.95}\\
    \footnotesize{\textit{47024}}& $D_1$ & & 60.72 & \tblue{96.00} & 79.75\\
    \midrule
    &$S$ &89.55 & 81.05 & 94.80&\tblue{95.42} \\
    Fridge&$D_0$ & 25.73& 55.28&  88.53 &\tblue{89.95} \\
    \footnotesize{\textit{11304}}&  $D_1$ &45.31 & 61.19& 80.48& \tblue{91.42}\\
      \bottomrule
    \end{tabular}}
        % \vspace{-2.5mm}
        \label{tab:comparison-ps2}
    \end{minipage}
    \hspace{5mm}
    \begin{minipage}[b]{0.45\linewidth}
    \centering
        \caption{\textbf{Results of complex objects} across 10 trials. For movable parts, we report the average.}
        \vspace{-2mm}
        \resizebox{1\textwidth}{!}{ 
    \begin{tabular}{c|c|c|c|c}
    \toprule
    &3D IoU ($\%$) & DTA & ArtGS & Ours\\
    \midrule
     \multirow{3}*{\textit{$\text{Storage}_{\text{47648}}$}}& $S$ & 87.95 & 93.32 &\tblue{97.01}\\
    & $D_{avg}$ & 26.38 & 52.23 &\tblue{79.34}\\
    & Mean &  35.18 & 58.14 &\tblue{81.87}\\
    \midrule
    \multirow{3}*{\textit{$\text{Table}_{\text{31249}}$}}& $S$ & 89.81& 90.44& \tblue{91.75}\\
    & $D_{avg}$ & 37.29 & 38.07 & \tblue{43.92}\\
    & Mean & 47.80& 48.55& \tblue{53.49}\\
      \bottomrule
    \end{tabular}}
    \label{tab:comparison-ps3}
    \end{minipage}
    \vspace{-5pt}
\end{table}

\begin{table}[t]
\centering
    \caption{\textbf{Quantitative evaluation of mesh reconstruction on two-part objects}. Lower ($\downarrow$) indicates better performance. $F$ indicates the failure.
}
    \label{tab:comparison-mr1}
    \resizebox{1\textwidth}{!}{ 
    \begin{tabular}{c|c|c|c|c|c|c|c|c}
    \toprule
    \multirow{2}*{Metric} & \multirow{2}*{Method}& \multicolumn{7}{c}{Two-part objects}\\
    \cmidrule{3-9}
    & &Fridge& Oven& Scissor& USB& Washer& Blade& Storage\\
    \midrule
    \rowcolor{gray!20}
    \multirow{5}{*}{\cellcolor{white}CD-s}& PARIS &2.85$_{\pm0.39}$ & 11.06$_{\pm1.86}$ & 2.31$_{\pm2.05}$  & F& 18.93$_{\pm 0.90}$ & 0.57$_{\pm0.02}$& 10.01$_{\pm0.58}$ \\
        \rowcolor{gray!20}
    \cellcolor{white}&  DTA &{3.19$_{\pm0.80}$} & {9.10$_{\pm3.59}$}& 9.41$_{\pm1.00}$& {2.04$_{\pm0.12}$} & {5.03$_{\pm3.44}$}& {0.33$_{\pm0.00}$} & {4.94$_{\pm0.14}$}\\
        \rowcolor{gray!20}
    \cellcolor{white}& ArtGS &{1.58$_{\pm0.28}$} & {8.39$_{\pm0.29}$}& {0.80$_{\pm0.99}$} & 11.01$_{\pm0.43}$& {6.63$_{\pm0.17}$}& {1.23$_{\pm0.01}$} & 7.50$_{\pm0.15}$\\
    \cellcolor{white}& Ours-b & 4.73$_{\pm0.53}$& 10.08$_{\pm1.43}$  & 2.22$_{\pm1.07}$ & 34.61$_{\pm1.73}$  & F& 1.90$_{\pm0.06}$& 7.27 $_{\pm0.78}$\\
    \cellcolor{white}& Ours &3.45$_{\pm0.09}$& 10.36$_{\pm0.73}$& \tblue{0.14$_{\pm0.00}$}& \tblue{1.54$_{\pm0.14}$}& 9.25$_{\pm0.99}$ & 1.76$_{\pm0.02}$& 7.09$_{\pm0.49}$ \\
    \midrule
        \rowcolor{gray!20}
    \multirow{5}*{CD-m}\cellcolor{white}& PARIS  &438.06$_{\pm52.16}$ & 856.81$_{\pm128.16}$& 35.61$_{\pm27.35}$ & F& 680.08$_{\pm34.40}$& 43.91$_{\pm12.25}$& 73.64$_{\pm4.67}$\\
        \rowcolor{gray!20}
    \cellcolor{white}&  DTA &{4.08$_{\pm0.60}$}& 77.61$_{\pm86.59}$& 141.99$_{\pm35.39}$& {1.90$_{\pm0.51}$} & 481.06$_{\pm66.34}$&{19.30$_{\pm2.09}$}&  67.33$_{\pm3.03}$ \\
        \rowcolor{gray!20}
    \cellcolor{white}& ArtGS &43.51$_{\pm0.47}$  & 64.34$_{\pm3.66}$&{53.71$_{\pm28.82}$} & 50.00$_{\pm19.77}$ & {155.65$_{\pm22.79}$}& 473.72$_{\pm7.62}$  & {6.92$_{\pm0.54}$} \\
    \cellcolor{white}& Ours-b & 18.27$_{\pm4.22}$& {5.17$_{\pm2.54}$} & 73.13$_{\pm50.33}$& 19.46$_{\pm0.46}$ & F & 110.46$_{\pm36.00}$& 88.85$_{\pm73.10}$ \\
    \cellcolor{white}& Ours &\tblue{2.21$_{\pm0.18}$}&\tblue{1.63$_{\pm0.25}$}&\tblue{0.27$_{\pm0.03}$} & \tblue{0.89$_{\pm0.10}$} &  \tblue{21.03 $_{\pm1.02}$}&\tblue{2.36$_{\pm0.09}$} &18.95$_{\pm2.57}$ \\
      \bottomrule
    \end{tabular}}
\end{table}
\begin{table}[t]
\centering
\vspace{-5pt}
    \begin{minipage}[b]{0.45\linewidth}
    \centering
        \caption{\textbf{Performance on three-part objects.} we report the CD distance (\textit{mm}) (mean over 10 trials).}
        \vspace{-2mm}
        \resizebox{1\textwidth}{!}{ 
    \begin{tabular}{c|c|c|c|c|c}
    \toprule
    & $\downarrow$&PARIS-m &DTA & ArtGS & Ours\\
    \midrule
    & CD-s & 8.05  & \tblue{3.20} & 3.58  & 10.37 \\
    Storage& CD-m ($D_0$) &  \multirow{2}*{F}& 275.87 & 253.69 &\tblue{0.81}\\
    \footnotesize{\textit{47024}}& CD-m ($D_1$) &  & 287.70 & \tblue{1.21} & 27.35\\
    \midrule
    & CD-s & 6.91 & 4.90 & \tblue{2.93} & 8.16 \\
    Fridge& CD-m ($D_0$) &298.29 &29.95 & 12.83   & \tblue{3.85}\\
    \footnotesize{\textit{11304}}&  CD-m ($D_1$)&189.85 &323.06 &12.17 &  \tblue{2.12}\\
      \bottomrule
    \end{tabular}}
        % \vspace{-2.5mm}
        \label{tab:comparison-mr2}
    \end{minipage}
    \hspace{5mm}
    \begin{minipage}[b]{0.45\linewidth}
    \centering
        \caption{\textbf{Complex objects}: average CD distance for movable parts across 10 trials.}
        \vspace{-2mm}
        \resizebox{1\textwidth}{!}{ 
    \begin{tabular}{c|c|c|c|c}
    \toprule
    & $\downarrow$ & DTA & ArtGS & Ours\\
    \midrule
     \multirow{2}*{\textit{$\text{Storage}_{\text{47648}}$}}& CD-s & \tblue{2.08} &2.96 & 2.63 \\
    & CD-m$_{avg}$& 200.15 & 71.17& \tblue{8.36}\\
    \midrule
    \multirow{2}*{\textit{$\text{Table}_{\text{31249}}$}}& CD-s & \tblue{2.56} & 3.65 &  3.08 \\
    & CD-m$_{avg}$& 152.93 & 51.40& \tblue{4.99}\\
    \bottomrule
    \end{tabular}}
    \label{tab:comparison-mr3}
    \end{minipage}
    \vspace{-5pt}
\end{table}

\begin{table}[t]
    \caption{\textbf{Quantitative evaluation on PARIS-ours dataset}. We report the metrics over 10 trials as mean$\pm$std. Ours-b failed on the laptop and washer, and PARIS failed onthe  stapler and USB, denoted as $F$. $-$ indicates that prismatic type joints have no rotation axis. Highlighting: All metrics lower is better, and we highlight \tblue{best} and \tbrown{second-best} results.
}
    \label{tab:comparison-to-soat}
    
    \resizebox{1\textwidth}{!}{ 
    \begin{tabular}{c|c|c|c|c|c|c|c|c|c|c|c}
    \toprule
    \multirow{2}*{Metric} & \multirow{2}*{Method}& \multicolumn{10}{c}{PARIS-dataset}\\
    \cmidrule{3-12}
    & & FoldChair&Fridge&Laptop& Oven& Scissor&Stapler& USB& Washer& Blade& Storage\\
    \midrule
    & PARIS & 10.52$_{\pm9.77}$ & 66.19$_{\pm25.37}$ & 7.75$_{\pm8.60}$ & 19.58$_{\pm21.20}$ & 31.29$_{\pm21.89}$ & F & F & 14.88$_{\pm15.81}$ &  2.58$_{\pm0.87}$ & 9.64$_{\pm1.37}$\\
    Axis& DTA & \tbrown{0.03$_{\pm0.01}$}&\tblue{1.86$_{\pm3.38}$}&\tbrown{0.89$_{\pm0.93}$} & 5.39$_{\pm7.16}$ & \tblue{1.01$_{\pm1.23}$}& \tblue{0.17$_{\pm0.12}$}& \tblue{0.22$_{\pm0.11}$}& \tbrown{17.34$_{\pm25.59}$} & 1.65$_{\pm0.35}$ &8.18$_{\pm6.80}$ \\
    Ang& ArtGS & \tblue{0.00$_{\pm0.00}$} & 89.18$_{\pm0.02}$ & \tblue{0.00$_{\pm0.00}$} & 89.92$_{\pm0.04}$ & 2.39$_{\pm1.91}$ & 9.70$_{\pm21.17}$ & 23.86$_{\pm35.02}$ & 37.48$_{\pm40.08}$ & 1.31$_{\pm0.14}$ & \tblue{0.00$_{\pm0.01}$} \\
    & Ours-b &0.92$_{\pm0.46}$&6.76$_{\pm3.40}$& F& \tbrown{3.36$_{\pm3.31}$}  & 5.12$_{\pm0.46}$ &45.15$_{\pm27.07}$&6.65$_{\pm4.20}$  &F &\tblue{0.25$_{\pm4.20}$} & 1.72$_{\pm0.67}$\\
    & Ours &0.21$_{\pm0.07}$& \tbrown{2.70$_{\pm1.73}$}& 1.73$_{\pm1.36}$& \tblue{0.27$_{\pm0.25}$}&\tbrown{1.60$_{\pm0.38}$} & \tbrown{0.91$_{\pm0.64}$}& \tbrown{0.59$_{\pm0.30}$}& \tblue{1.63$_{\pm0.90}$}&\tbrown{0.18$_{\pm0.17}$} & \tbrown{1.38$_{\pm0.96}$} \\
    \midrule
    & PARIS & 0.44$_{\pm0.39}$ & \tblue{0.68$_{\pm1.01}$} & 1.20$_{\pm1.09}$ & 3.04$_{\pm2.60}$ & 1.07$_{\pm1.40}$ & F & F & \tbrown{2.67$_{\pm2.40}$} & $-$ & $-$ \\
    Axis&  DTA &\tbrown{0.01$_{\pm0.00}$} & 2.86$_{\pm2.45}$ & 1.75$_{\pm1.20}$&4.98$_{\pm4.38}$  &8.84$_{\pm4.76}$& 11.64$_{\pm2.55}$& \tblue{0.01$_{\pm0.01}$} &26.50$_{\pm42.41}$&$-$ & $-$\\
    Pos& ArtGS & \tblue{0.00$_{\pm0.00}$} & 1.54$_{\pm0.00}$ & \tblue{0.00$_{\pm0.00}$} & 2.12$_{\pm0.07}$ & 1.73$_{\pm1.70}$ & \tbrown{2.82$_{\pm6.35}$} & 6.01$_{\pm8.60}$ & 4.35$_{\pm1.52}$ & $-$ & $-$ \\
    & Ours-b &0.05$_{\pm0.03}$&1.22$_{\pm0.86}$& F& \tbrown{1.24$_{\pm0.86}$} &\tbrown{0.86$_{\pm0.55}$} & 11.39$_{\pm5.17}$& \tbrown{0.84$_{\pm0.37}$}& F &$-$& $-$ \\
    & Ours &0.04$_{\pm0.01}$&\tbrown{1.21$_{\pm0.20}$}&\tbrown{0.86$_{\pm0.34}$} &\tblue{1.13$_{\pm0.68}$} & \tblue{0.75$_{\pm0.05}$}& \tblue{1.43$_{\pm0.77}$}& 1.45$_{\pm0.71}$ & \tblue{1.12$_{\pm0.29}$}&$-$& $-$\\
     \midrule
    & PARIS & 178.21$_{\pm1.54}$ & 118.14$_{\pm29.33}$ & 167.60$_{\pm14.49}$ & 144.80$_{\pm11.20}$ & 122.05$_{\pm42.50}$ & F & F & 86.13$_{\pm3.11}$ & 0.08$_{\pm0.06}$ & 0.10$_{\pm0.02}$\\
    Part&  DTA &\tbrown{0.10$_{\pm0.02}$}& 177.48$_{\pm20.68}$& 171.77$_{\pm13.43}$ & 142.10$_{\pm33.62}$& 150.50$_{\pm11.29}$& 177.80$_{\pm0.72}$&\tblue{0.32$_{\pm0.15}$} & 76.43$_{\pm11.27}$ & 0.02$_{\pm0.00}$ & 0.07$_{\pm0.06}$\\
    Motion& ArtGS & \tblue{0.01$_{\pm0.01}$} & 110.00$_{\pm0.00}$ & \tblue{0.02$_{\pm0.01}$} & 90.00$_{\pm0.00}$ & 99.09$_{\pm67.18}$ & \tbrown{17.98$_{\pm31.01}$} & 120.05$_{\pm19.63}$ & \tbrown{74.42$_{\pm10.42}$} & 0.14$_{\pm0.00}$ & \tblue{0.00$_{\pm0.00}$} \\
    & Ours-b &2.60$_{\pm1.09}$&\tbrown{16.16$_{\pm11.76}$}&F& \tbrown{11.38$_{\pm9.35}$}& \tbrown{11.50$_{\pm3.73}$}& 137.47$_{\pm44.85}$& 30.90$_{\pm4.68}$& F&  \tbrown{0.01$_{\pm0.00}$}&0.03$_{\pm0.01}$ \\
    & Ours &1.84$_{\pm0.38}$&\tblue{5.10$_{\pm2.31}$}& \tbrown{10.67$_{\pm3.49}$}& \tblue{7.64$_{\pm1.77}$} &\tblue{5.20$_{\pm0.40}$}& \tblue{9.08$_{\pm1.84}$} & \tbrown{16.94$_{\pm1.85}$}&\tblue{6.90$_{\pm2.88}$} &\tblue{0.01$_{\pm0.00}$} & \tbrown{0.02$_{\pm0.01}$}\\
      \midrule
      \multirow5*{CD-s}& PARIS & 6.03$_{\pm3.72}$ &2.85$_{\pm0.39}$ & 0.77$_{\pm0.71}$ & 11.06$_{\pm1.86}$ & 2.31$_{\pm2.05}$  &F& F& 18.93$_{\pm 0.90}$ & 0.57$_{\pm0.02}$& 10.01$_{\pm0.58}$ \\
    &  DTA &\tbrown{0.18$_{\pm0.01}$}&\tbrown{3.19$_{\pm0.80}$}&2.75$_{\pm5.36}$ & \tbrown{9.10$_{\pm3.59}$}& 9.41$_{\pm1.00}$& 3.13$_{\pm0.06}$& \tbrown{2.04$_{\pm0.12}$} & \tblue{5.03$_{\pm3.44}$}& \tblue{0.33$_{\pm0.00}$} & \tblue{4.94$_{\pm0.14}$}\\
    & ArtGS & 0.96$_{\pm1.62}$ &\tblue{1.58$_{\pm0.28}$} &\tblue{0.12$_{\pm0.00}$}& \tblue{8.39$_{\pm0.29}$}& \tbrown{0.80$_{\pm0.99}$} & \tblue{1.18$_{\pm0.42}$} & 11.01$_{\pm0.43}$& \tbrown{6.63$_{\pm0.17}$}& \tbrown{1.23$_{\pm0.01}$} & 7.50$_{\pm0.15}$\\
    & Ours-b & 3.05$_{\pm0.16}$ &4.73$_{\pm0.53}$&F& 10.08$_{\pm1.43}$  & 2.22$_{\pm1.07}$ & 104.12$_{\pm18.45}$ &34.61$_{\pm1.73}$  & F& 1.90$_{\pm0.06}$& 7.27 $_{\pm0.78}$\\
    & Ours &\tblue{0.16$_{\pm0.00}$}&3.45$_{\pm0.09}$&\tbrown{0.46$_{\pm0.08}$}& 10.36$_{\pm0.73}$& \tblue{0.14$_{\pm0.00}$}& \tbrown{1.71$_{\pm 0.24}$}& \tblue{1.54$_{\pm0.14}$}& 9.25$_{\pm0.99}$ & 1.76$_{\pm0.02}$& \tbrown{6.44$_{\pm0.06}$}\\
      \midrule
      \multirow{5}*{CD-m}& PARIS & 3.68$_{\pm2.31}$ &438.06$_{\pm52.16}$ & 331.47$_{\pm19.66}$ & 856.81$_{\pm128.16}$& 35.61$_{\pm27.35}$ &F& F& 680.08$_{\pm34.40}$& 43.91$_{\pm12.25}$& 73.64$_{\pm4.67}$\\
    &  DTA &\tblue{0.13$_{\pm0.00}$}&\tbrown{4.08$_{\pm0.60}$}&\tbrown{1.34$_{\pm1.67}$} & 77.61$_{\pm86.59}$& 141.99$_{\pm35.39}$& 8.41$_{\pm0.55}$& \tbrown{1.90$_{\pm0.51}$} & 481.06$_{\pm66.34}$&\tbrown{19.30$_{\pm2.09}$}&  67.33$_{\pm3.03}$ \\
    & ArtGS &\tbrown{0.26$_{\pm0.19}$} &43.51$_{\pm0.47}$ &\tblue{0.13$_{\pm0.00}$} & 64.34$_{\pm3.66}$&\tbrown{53.71$_{\pm28.82}$} & \tblue{0.93$_{\pm0.45}$}& 50.00$_{\pm19.77}$ & \tbrown{155.65$_{\pm22.79}$}& 473.72$_{\pm7.62}$  & \tblue{6.92$_{\pm0.54}$} \\
    & Ours-b &1.30$_{\pm1.60}$ & 18.27$_{\pm4.22}$&F& \tbrown{5.17$_{\pm2.54}$} & 73.13$_{\pm50.33}$& 11.72$_{\pm8.60}$& 19.46$_{\pm0.46}$ & F & 110.46$_{\pm36.00}$& 88.85$_{\pm73.10}$ \\
    & Ours & 0.45$_{\pm0.02}$&\tblue{2.21$_{\pm0.18}$}&2.01$_{\pm0.19}$& \tblue{1.63$_{\pm0.25}$}&\tblue{0.27$_{\pm0.03}$} & \tbrown{1.68$_{\pm0.75}$ }&\tblue{0.89$_{\pm0.10}$} &  \tblue{21.03 $_{\pm1.02}$}&\tblue{2.36$_{\pm0.09}$} & \tbrown{22.33$_{\pm1.47}$}\\
      \midrule
      \multirow{5}*{CD-w}& PARIS &1.31$_{\pm0.40}$&30.75$_{\pm10.37}$ & 48.07$_{\pm7.25}$& 27.24$_{\pm2.98}$ & 2.82$_{\pm1.49}$ &F & F&23.20$_{\pm0.84}$ & \tbrown{1.26$_{\pm0.05}$} & 11.59$_{\pm0.27}$\\
    &  DTA &\tblue{0.26$_{\pm0.00}$}& \tbrown{2.10$_{\pm0.08}$}& \tbrown{0.33$_{\pm0.00}$}&\tblue{5.76$_{\pm0.09}$} & 0.42 $_{\pm0.01}$& 1.98$_{\pm0.02}$ & \tbrown{1.12$_{\pm0.01}$} &\tblue{3.97$_{\pm0.09}$}& \tblue{0.29$_{\pm0.00}$} & \tblue{4.67$_{\pm0.06}$}\\
    & ArtGS &\tbrown{0.74$_{\pm0.99}$} & \tblue{1.91$_{\pm0.07}$} & \tblue{0.23$_{\pm0.00}$} & 9.01$_{\pm0.23}$& 4.53$_{\pm1.59}$ &\tblue{1.21$_{\pm0.55}$} & 11.76$_{\pm0.51}$& \tbrown{7.43$_{\pm0.13}$} & 1.28$_{\pm0.29}$ & \tbrown{5.67$_{\pm0.15}$}\\
    & Ours-b & 0.34$_{\pm0.00}$ & 3.76$_{\pm0.12}$&F& \tbrown{8.32$_{\pm0.22}$} &\tblue{0.26$_{\pm0.05}$} &1.62$_{\pm0.13}$ & 1.13$_{\pm0.07}$& F & 1.54$_{\pm0.01}$ & 7.28 $_{\pm2.75}$ \\
    & Ours &0.38$_{\pm0.01}$&4.31$_{\pm0.10}$& 1.32$_{\pm0.12}$& 8.66$_{\pm0.44}$&\tbrown{0.26$_{\pm0.01}$} & \tbrown{1.30$_{\pm0.21}$} & \tblue{1.06$_{\pm0.07}$}& 9.44$_{\pm0.49}$&1.73$_{\pm0.01}$ & 5.86$_{\pm0.13}$\\
      \bottomrule
    \end{tabular}}
\end{table}
\begin{table}[t]
    \caption{\textbf{Quantitative evaluation on DTA-multi (with two moving parts) dataset}. We follow~\citep{weng2024neural,liu2025building} to obtain the metrics over 10 trials and report them as mean$\pm$std.
}
    \label{tab:comparison-to-soat}
    
    \resizebox{1\textwidth}{!}{ 
    \begin{tabular}{c|c|c|c|c|c|c|c|c|c|c|c}
    \toprule
    \multirow{2}*{}& \multirow{2}*{Method} &  \multicolumn{4}{c|}{Part-0}&  \multicolumn{4}{c|}{Part-1} &\multirow{2}*{CD-s} & \multirow{2}*{CD-w}\\
        \cmidrule{3-10}
      & &  Axis Ang&Axis Pose & Part Motion &CD-m&  Axis Ang&Axis Pose & Part Motion &CD-m& & \\
      \midrule
      \multirow{4}*{Fridge}& PARIS-m &21.27$_{\pm12.67}$ &2.30$_{\pm3.09}$&46.45$_{\pm11.63}$ &131.92$_{\pm48.64}$&73.26$_{\pm13.81}$&0.49$_{\pm0.40}$&166.29$_{\pm 14.79}$  &639.12$_{\pm54.42}$&5.17$_{\pm 0.95}$ &6.39$_{\pm 0.84}$\\
      & DTA & 1.55$_{\pm1.22}$ &\textbf{0.69$_{\pm1.05}$} & 14.33$_{\pm15.14}$ & 18.03$_{\pm6.02}$ &13.08$_{\pm3.23}$  & 94.98$_{\pm74.37}$ &  173.92$_{\pm8.77}$ & 220.55$_{\pm42.04}$ & 3.61$_{\pm0.53}$ & \textbf{2.03$_{\pm0.01}$}\\
      & ArtGS & 13.94$_{\pm9.59}$  &46.95$_{\pm12.83}$&176.52$_{\pm1.04}$&  11.80$_{\pm4.01}$ &3.33$_{\pm1.33}$&15.79$_{\pm6.24}$&41.81$_{\pm4.22}$& 11.24$_{\pm1.91}$ & \textbf{0.98$_{\pm0.19}$}&2.07$_{\pm0.21}$ \\
       & Ours & \textbf{0.68$_{\pm0.31}$} &3.58$_{\pm1.04}$& \textbf{3.57$_{\pm1.74}$}&\textbf{3.85$_{\pm1.61}$}& \textbf{1.67$_{\pm0.62}$}& \textbf{0.68$_{\pm0.47}$}&\textbf{ 4.81$_{\pm1.71}$} & \textbf{2.12$_{\pm1.39}$}& 8.16$_{\pm0.38}$ &5.40$_{\pm0.22}$ \\
        \midrule
     \multirow{4}*{Storage}& PARIS-m &F  &F&F &F&F&$-$&F  &F&F &F\\
      & DTA & 38.98$_{\pm 16.26}$  & 7.16$_{\pm2.24}$  &89.25$_{\pm2.39}$ &363.68$_{\pm102.26}$ & \textbf{0.24$_{\pm0.07}$} &$-$&\textbf{0.00$_{\pm0.00}$} & 221.74$_{\pm28.91}$ & \textbf{3.02$_{\pm0.14}$}  & \textbf{1.91$_{\pm0.03}$}\\
      & ArtGS &20.63$_{\pm6.83}$  &3.83$_{\pm2.03}$&107.56$_{\pm1.89}$ &252.69$_{\pm14.57}$&1.75$_{\pm1.50}$ &$-$&0.13$_{\pm0.12}$  &\textbf{1.26$_{\pm0.30}$}&3.76$_{\pm0.56}$ & 3.51$_{\pm0.40}$\\
       & Ours & \textbf{0.56$_{\pm0.77}$} & \textbf{1.26$_{\pm0.74}$} & \textbf{1.66$_{\pm1.04}$}& \textbf{0.81$_{\pm0.06}$} &1.03$_{\pm0.89}$& $-$& 0.06$_{\pm0.05}$& 27.35$_{\pm15.99}$& 10.37$_{\pm0.92}$ &6.87$_{\pm0.21}$\\
      \bottomrule
    \end{tabular}}
\end{table}

\begin{table}[htbp]
\caption{Motion type and motion records across ten scenes on PARIS dataset}
\label{tab:scene_motion}
\centering
\setlength{\tabcolsep}{6pt}

\resizebox{1\textwidth}{!}{ \begin{tabular}{l*{10}{c}}
\toprule
Scene        & FoldChair&Fridge&Laptop& Oven& Scissor&Stapler& USB& Washer& Blade& Storage \\
\midrule
Type  &Rotate&Rotate&Rotate&Rotate&Rotate&Rotate &Rotate &Rotate &Translate&Translate\\
Motion& [0.0, -80.0]&[-110.0, -0.0]&[90.0,0.0]&[0.0,90.0]&[45.0, -45.0]&[0.0, -80.0]&[0.0,-90.0]&[0.0,-60.0]&[0.0, 0.5]&[0.0, 0.5]\\
\bottomrule
\end{tabular}}
\end{table}

\begin{table}[t]
    \caption{\textbf{Quantitative evaluation of articulation estimation on two-part objects}. Lower ($\downarrow$) indicates better performance. $F$ indicates the failure. $-$ indicates that prismatic type joints have no rotation axis. Highlighting: \tblue{best}.
}
    \label{tab:comparison-mr1}
    \resizebox{1\textwidth}{!}{ 
    \begin{tabular}{c|c|c|c|c|c|c|c|c}
    \toprule
    \multirow{2}*{Metric} & \multirow{2}*{Method}& \multicolumn{7}{c}{Two-part objects}\\
    \cmidrule{3-9}
    & &Fridge& Oven& Scissor& USB& Washer& Blade& Storage\\
    \midrule
    & PARIS & 66.19$_{\pm25.37}$ & 19.58$_{\pm21.20}$ & 31.29$_{\pm21.89}$  & F & 14.88$_{\pm15.81}$ &  2.58$_{\pm0.87}$ & 9.64$_{\pm1.37}$\\

    Axis& DTA &{1.86$_{\pm3.8}$} & 5.39$_{\pm7.16}$ & {1.01$_{\pm1.23}$}& {0.22$_{\pm0.11}$}& {17.34$_{\pm25.59}$} & 1.65$_{\pm0.35}$ &8.18$_{\pm6.80}$ \\
    Ang& ArtGS & {89.91$_{\pm0.04}$} & 89.92$_{\pm0.04}$ & 2.39$_{\pm1.91}$ &  23.86$_{\pm35.02}$ & 37.48$_{\pm40.08}$ & 1.31$_{\pm0.14}$ & {0.00$_{\pm0.01}$} \\
    \rowcolor{gray!20}
    \cellcolor{white}& Ours-b & 6.76$_{\pm3.40}$& {3.36$_{\pm3.31}$}  & 5.12$_{\pm0.46}$ &6.65$_{\pm4.20}$  &F &{0.25$_{\pm4.20}$} & 1.72$_{\pm0.67}$\\
     \rowcolor{gray!20}
    \cellcolor{white}& Ours & 2.70$_{\pm1.73}$& \tblue{0.27$_{\pm0.25}$}&{1.60$_{\pm0.38}$} & {0.59$_{\pm0.30}$}& \tblue{1.63$_{\pm0.90}$}&\tblue{0.18$_{\pm0.17}$} & {1.52$_{\pm0.88}$} \\
    \midrule
    & PARIS & 1.20$_{\pm1.09}$ & 3.04$_{\pm2.60}$ & 1.07$_{\pm1.40}$ & F & {2.67$_{\pm2.40}$} & $-$ & $-$ \\
    Axis&  DTA & 1.75$_{\pm1.20}$&4.98$_{\pm4.38}$  &8.84$_{\pm4.76}$& {0.01$_{\pm0.01}$} &26.50$_{\pm42.41}$&$-$ & $-$\\
    Pos& ArtGS & {1.54$_{\pm0.00}$} & 2.12$_{\pm0.07}$ & 1.73$_{\pm1.70}$ &  6.01$_{\pm8.60}$ & 4.35$_{\pm1.52}$ & $-$ & $-$ \\
     \rowcolor{gray!20}
    \cellcolor{white}& Ours-b & 1.22$_{\pm0.86}$& {1.24$_{\pm0.86}$} &\tblue{{0.86$_{\pm0.55}$}} &  {0.84$_{\pm0.37}$}& F &$-$& $-$ \\
     \rowcolor{gray!20}
    \cellcolor{white}& Ours &\textbf{{0.86$_{\pm0.34}$}} &\tblue{1.13$_{\pm0.68}$} & \tblue{0.75$_{\pm0.05}$}& 1.45$_{\pm0.71}$ & \tblue{1.12$_{\pm0.29}$}&$-$& $-$\\
     \midrule
    & PARIS & 167.60$_{\pm14.49}$ & 144.80$_{\pm11.20}$ & 122.05$_{\pm42.50}$ & F & 86.13$_{\pm3.11}$ & 0.08$_{\pm0.06}$ & 0.10$_{\pm0.02}$\\
    Part&  DTA & 171.77$_{\pm13.43}$ & 142.10$_{\pm33.62}$& 150.50$_{\pm11.29}$&{0.32$_{\pm0.15}$} & 76.43$_{\pm11.27}$ & 0.02$_{\pm0.00}$ & 0.07$_{\pm0.06}$\\
    Motion& ArtGS & {110.00$_{\pm0.00}$} & 90.00$_{\pm0.00}$ & 99.09$_{\pm67.18}$ & 120.05$_{\pm19.63}$ & {74.42$_{\pm10.42}$} & 0.14$_{\pm0.00}$ & {0.00$_{\pm0.00}$} \\
     \rowcolor{gray!20}
   \cellcolor{white} & Ours-b &16.16$_{\pm11.76}$& {11.38$_{\pm9.35}$}& {11.50$_{\pm3.73}$}& 30.90$_{\pm4.68}$& F&  {0.01$_{\pm0.00}$}&0.03$_{\pm0.01}$ \\
     \rowcolor{gray!20}
   \cellcolor{white} & Ours & \tblue{{10.67$_{\pm3.49}$}}& \tblue{7.64$_{\pm1.77}$} &\tblue{5.20$_{\pm0.40}$}& {16.94$_{\pm1.85}$}&\tblue{6.90$_{\pm2.88}$} &\tblue{0.01$_{\pm0.00}$} & \tblue{0.02$_{\pm0.00}$} \\
      \bottomrule
    \end{tabular}}
\end{table}
\begin{table}[t]
\centering
\vspace{-5pt}
    \begin{minipage}[t]{0.65\linewidth}
    \centering
        \caption{\textbf{Quantitative comparison on three-part objects.} The results are reported as the mean over 10 trials.}
        \vspace{-2mm}
        \resizebox{1\textwidth}{!}{ 
    \begin{tabular}{c|c|c|c|c|c|c|c}
    \toprule
    & \multirow{2}*{Methods} & \multicolumn{3}{c|}{$D_0$} & \multicolumn{3}{c}{$D_1$}\\
    \cmidrule{3-8}
    &  & Axis Ang& Axis Pos & Part Motion& Axis Ang& Axis Pos & Part Motion\\
    \midrule
    
    & DTA& 58.63 & 38.59 & 96.56 & \tblue{0.50} & $-$& \tblue{0.01}\\
    Storage& ArtGS& 20.63 & 3.83& 107.56& 1.75 & $-$& 0.13\\
    \scriptsize{47024}& Ours& \tblue{0.56}&\tblue{1.26}  &\tblue{1.66}  & 1.03  &$-$ & 0.06 \\
    \midrule
    & DTA& 22.02 & 359.06 & 178.80 &  9.48 & 6.22 & 38.36\\
    Fridge& ArtGS& 13.94 & 46.95& 176.52& 3.33 & 15.79& 41.81\\
    \textit{\scriptsize{11304}}& Ours& \tblue{0.68}&  \tblue{3.58}& \tblue{3.57} & \tblue{ 1.67} &\tblue{0.68} & \tblue{4.81}\\
      \bottomrule
    \end{tabular}}
        % \vspace{-2.5mm}
        \label{tab:comparison-mr2}
    \end{minipage}
    \hspace{2mm}
    \begin{minipage}[t]{0.32\linewidth}
    \centering
        \caption{\textbf{Quantitative comparison on complex objects.}.}
        \vspace{-2mm}
        \resizebox{0.95\textwidth}{!}{ 
    \begin{tabular}{c|c|c|c}
    \toprule
    & $\downarrow$ & ArtGS & Ours\\
    \midrule
     & Ang$_{avg}$ & 12.78 & \tblue{0.58}\\
    Storage & Pose$_{avg}$  & 3.34& \tblue{1.31}\\
    \textit{\scriptsize{47648}}& Motion$^{r}_{avg}$   & 81.93 &\tblue{10.56}
\\
    & Motion$^{p}_{avg}$   & 0.18 & \tblue{0.02}
\\
    \midrule
    & Ang$_{avg}$ & 33.19 & \tblue{1.19}\\
    Table& Pose$_{avg}$&  2.42& \tblue{0.81}\\
    \textit{\scriptsize{31249}}& Motion$^{r}_{avg}$ & 82.29 & \tblue{1.10}\\
    & Motion$^{p}_{avg}$   & 0.43& \tblue{0.01}\\
    \bottomrule
    \end{tabular}}
    \label{tab:comparison-mr3}
    \end{minipage}
    \vspace{-5pt}
\end{table}
\begin{table}[t]
    \caption{\textbf{Quantitative evaluation on PARIS-ours dataset}. We report the metrics over 10 trials as mean$\pm$std. Ours-b failed on the laptop and washer, and PARIS failed onthe  stapler and USB, denoted as $F$. $-$ indicates that prismatic type joints have no rotation axis. Highlighting: All metrics lower is better, and we highlight \tblue{best} and \tbrown{second-best} results.
}
    \label{tab:comparison-to-soat}
    
    \resizebox{1\textwidth}{!}{ 
    \begin{tabular}{c|c|c|c|c|c|c|c|c|c|c|c}
    \toprule
    \multirow{2}*{Metric} & \multirow{2}*{Method}& \multicolumn{10}{c}{PARIS-dataset}\\
    \cmidrule{3-12}
    & & FoldChair&Fridge&Laptop& Oven& Scissor&Stapler& USB& Washer& Blade& Storage\\
    \midrule
    & PARIS & 10.52$_{\pm9.77}$ & 66.19$_{\pm25.37}$ & 7.75$_{\pm8.60}$ & 19.58$_{\pm21.20}$ & 31.29$_{\pm21.89}$ & F & F & 14.88$_{\pm15.81}$ &  2.58$_{\pm0.87}$ & 9.64$_{\pm1.37}$\\
    Axis& DTA & \tbrown{0.03$_{\pm0.01}$}&\tblue{1.86$_{\pm3.38}$}&\tbrown{0.89$_{\pm0.93}$} & 5.39$_{\pm7.16}$ & \tblue{1.01$_{\pm1.23}$}& \tblue{0.17$_{\pm0.12}$}& \tblue{0.22$_{\pm0.11}$}& \tbrown{17.34$_{\pm25.59}$} & 1.65$_{\pm0.35}$ &8.18$_{\pm6.80}$ \\
    Ang& ArtGS & \tblue{0.00$_{\pm0.00}$} & 89.18$_{\pm0.02}$ & \tblue{0.00$_{\pm0.00}$} & 89.92$_{\pm0.04}$ & 2.39$_{\pm1.91}$ & 9.70$_{\pm21.17}$ & 23.86$_{\pm35.02}$ & 37.48$_{\pm40.08}$ & 1.31$_{\pm0.14}$ & \tblue{0.00$_{\pm0.01}$} \\
    & Ours-b &0.92$_{\pm0.46}$&6.76$_{\pm3.40}$& F& \tbrown{3.36$_{\pm3.31}$}  & 5.12$_{\pm0.46}$ &45.15$_{\pm27.07}$&6.65$_{\pm4.20}$  &F &\tblue{0.25$_{\pm4.20}$} & 1.72$_{\pm0.67}$\\
    & Ours &0.21$_{\pm0.07}$& \tbrown{2.70$_{\pm1.73}$}& 1.73$_{\pm1.36}$& \tblue{0.27$_{\pm0.25}$}&\tbrown{1.60$_{\pm0.38}$} & \tbrown{0.91$_{\pm0.64}$}& \tbrown{0.59$_{\pm0.30}$}& \tblue{1.63$_{\pm0.90}$}&\tbrown{0.18$_{\pm0.17}$} & \tbrown{1.38$_{\pm0.96}$} \\
    \midrule
    & PARIS & 0.44$_{\pm0.39}$ & \tblue{0.68$_{\pm1.01}$} & 1.20$_{\pm1.09}$ & 3.04$_{\pm2.60}$ & 1.07$_{\pm1.40}$ & F & F & \tbrown{2.67$_{\pm2.40}$} & $-$ & $-$ \\
    Axis&  DTA &\tbrown{0.01$_{\pm0.00}$} & 2.86$_{\pm2.45}$ & 1.75$_{\pm1.20}$&4.98$_{\pm4.38}$  &8.84$_{\pm4.76}$& 11.64$_{\pm2.55}$& \tblue{0.01$_{\pm0.01}$} &26.50$_{\pm42.41}$&$-$ & $-$\\
    Pos& ArtGS & \tblue{0.00$_{\pm0.00}$} & 1.54$_{\pm0.00}$ & \tblue{0.00$_{\pm0.00}$} & 2.12$_{\pm0.07}$ & 1.73$_{\pm1.70}$ & \tbrown{2.82$_{\pm6.35}$} & 6.01$_{\pm8.60}$ & 4.35$_{\pm1.52}$ & $-$ & $-$ \\
    & Ours-b &0.05$_{\pm0.03}$&1.22$_{\pm0.86}$& F& \tbrown{1.24$_{\pm0.86}$} &\tbrown{0.86$_{\pm0.55}$} & 11.39$_{\pm5.17}$& \tbrown{0.84$_{\pm0.37}$}& F &$-$& $-$ \\
    & Ours &0.04$_{\pm0.01}$&\tbrown{1.21$_{\pm0.20}$}&\tbrown{0.86$_{\pm0.34}$} &\tblue{1.13$_{\pm0.68}$} & \tblue{0.75$_{\pm0.05}$}& \tblue{1.43$_{\pm0.77}$}& 1.45$_{\pm0.71}$ & \tblue{1.12$_{\pm0.29}$}&$-$& $-$\\
     \midrule
    & PARIS & 178.21$_{\pm1.54}$ & 118.14$_{\pm29.33}$ & 167.60$_{\pm14.49}$ & 144.80$_{\pm11.20}$ & 122.05$_{\pm42.50}$ & F & F & 86.13$_{\pm3.11}$ & 0.08$_{\pm0.06}$ & 0.10$_{\pm0.02}$\\
    Part&  DTA &\tbrown{0.10$_{\pm0.02}$}& 177.48$_{\pm20.68}$& 171.77$_{\pm13.43}$ & 142.10$_{\pm33.62}$& 150.50$_{\pm11.29}$& 177.80$_{\pm0.72}$&\tblue{0.32$_{\pm0.15}$} & 76.43$_{\pm11.27}$ & 0.02$_{\pm0.00}$ & 0.07$_{\pm0.06}$\\
    Motion& ArtGS & \tblue{0.01$_{\pm0.01}$} & 110.00$_{\pm0.00}$ & \tblue{0.02$_{\pm0.01}$} & 90.00$_{\pm0.00}$ & 99.09$_{\pm67.18}$ & \tbrown{17.98$_{\pm31.01}$} & 120.05$_{\pm19.63}$ & \tbrown{74.42$_{\pm10.42}$} & 0.14$_{\pm0.00}$ & \tblue{0.00$_{\pm0.00}$} \\
    & Ours-b &2.60$_{\pm1.09}$&\tbrown{16.16$_{\pm11.76}$}&F& \tbrown{11.38$_{\pm9.35}$}& \tbrown{11.50$_{\pm3.73}$}& 137.47$_{\pm44.85}$& 30.90$_{\pm4.68}$& F&  \tbrown{0.01$_{\pm0.00}$}&0.03$_{\pm0.01}$ \\
    & Ours &1.84$_{\pm0.38}$&\tblue{5.10$_{\pm2.31}$}& \tbrown{10.67$_{\pm3.49}$}& \tblue{7.64$_{\pm1.77}$} &\tblue{5.20$_{\pm0.40}$}& \tblue{9.08$_{\pm1.84}$} & \tbrown{16.94$_{\pm1.85}$}&\tblue{6.90$_{\pm2.88}$} &\tblue{0.01$_{\pm0.00}$} & \tbrown{0.02$_{\pm0.01}$}\\
      \midrule
      \multirow5*{CD-s}& PARIS & 6.03$_{\pm3.72}$ &2.85$_{\pm0.39}$ & 0.77$_{\pm0.71}$ & 11.06$_{\pm1.86}$ & 2.31$_{\pm2.05}$  &F& F& 18.93$_{\pm 0.90}$ & 0.57$_{\pm0.02}$& 10.01$_{\pm0.58}$ \\
    &  DTA &\tbrown{0.18$_{\pm0.01}$}&\tbrown{3.19$_{\pm0.80}$}&2.75$_{\pm5.36}$ & \tbrown{9.10$_{\pm3.59}$}& 9.41$_{\pm1.00}$& 3.13$_{\pm0.06}$& \tbrown{2.04$_{\pm0.12}$} & \tblue{5.03$_{\pm3.44}$}& \tblue{0.33$_{\pm0.00}$} & \tblue{4.94$_{\pm0.14}$}\\
    & ArtGS & 0.96$_{\pm1.62}$ &\tblue{1.58$_{\pm0.28}$} &\tblue{0.12$_{\pm0.00}$}& \tblue{8.39$_{\pm0.29}$}& \tbrown{0.80$_{\pm0.99}$} & \tblue{1.18$_{\pm0.42}$} & 11.01$_{\pm0.43}$& \tbrown{6.63$_{\pm0.17}$}& \tbrown{1.23$_{\pm0.01}$} & 7.50$_{\pm0.15}$\\
    & Ours-b & 3.05$_{\pm0.16}$ &4.73$_{\pm0.53}$&F& 10.08$_{\pm1.43}$  & 2.22$_{\pm1.07}$ & 104.12$_{\pm18.45}$ &34.61$_{\pm1.73}$  & F& 1.90$_{\pm0.06}$& 7.27 $_{\pm0.78}$\\
    & Ours &\tblue{0.16$_{\pm0.00}$}&3.45$_{\pm0.09}$&\tbrown{0.46$_{\pm0.08}$}& 10.36$_{\pm0.73}$& \tblue{0.14$_{\pm0.00}$}& \tbrown{1.71$_{\pm 0.24}$}& \tblue{1.54$_{\pm0.14}$}& 9.25$_{\pm0.99}$ & 1.76$_{\pm0.02}$& \tbrown{6.44$_{\pm0.06}$}\\
      \midrule
      \multirow{5}*{CD-m}& PARIS & 3.68$_{\pm2.31}$ &438.06$_{\pm52.16}$ & 331.47$_{\pm19.66}$ & 856.81$_{\pm128.16}$& 35.61$_{\pm27.35}$ &F& F& 680.08$_{\pm34.40}$& 43.91$_{\pm12.25}$& 73.64$_{\pm4.67}$\\
    &  DTA &\tblue{0.13$_{\pm0.00}$}&\tbrown{4.08$_{\pm0.60}$}&\tbrown{1.34$_{\pm1.67}$} & 77.61$_{\pm86.59}$& 141.99$_{\pm35.39}$& 8.41$_{\pm0.55}$& \tbrown{1.90$_{\pm0.51}$} & 481.06$_{\pm66.34}$&\tbrown{19.30$_{\pm2.09}$}&  67.33$_{\pm3.03}$ \\
    & ArtGS &\tbrown{0.26$_{\pm0.19}$} &43.51$_{\pm0.47}$ &\tblue{0.13$_{\pm0.00}$} & 64.34$_{\pm3.66}$&\tbrown{53.71$_{\pm28.82}$} & \tblue{0.93$_{\pm0.45}$}& 50.00$_{\pm19.77}$ & \tbrown{155.65$_{\pm22.79}$}& 473.72$_{\pm7.62}$  & \tblue{6.92$_{\pm0.54}$} \\
    & Ours-b &1.30$_{\pm1.60}$ & 18.27$_{\pm4.22}$&F& \tbrown{5.17$_{\pm2.54}$} & 73.13$_{\pm50.33}$& 11.72$_{\pm8.60}$& 19.46$_{\pm0.46}$ & F & 110.46$_{\pm36.00}$& 88.85$_{\pm73.10}$ \\
    & Ours & 0.45$_{\pm0.02}$&\tblue{2.21$_{\pm0.18}$}&2.01$_{\pm0.19}$& \tblue{1.63$_{\pm0.25}$}&\tblue{0.27$_{\pm0.03}$} & \tbrown{1.68$_{\pm0.75}$ }&\tblue{0.89$_{\pm0.10}$} &  \tblue{21.03 $_{\pm1.02}$}&\tblue{2.36$_{\pm0.09}$} & \tbrown{22.33$_{\pm1.47}$}\\
      \midrule
      \multirow{5}*{CD-w}& PARIS &1.31$_{\pm0.40}$&30.75$_{\pm10.37}$ & 48.07$_{\pm7.25}$& 27.24$_{\pm2.98}$ & 2.82$_{\pm1.49}$ &F & F&23.20$_{\pm0.84}$ & \tbrown{1.26$_{\pm0.05}$} & 11.59$_{\pm0.27}$\\
    &  DTA &\tblue{0.26$_{\pm0.00}$}& \tbrown{2.10$_{\pm0.08}$}& \tbrown{0.33$_{\pm0.00}$}&\tblue{5.76$_{\pm0.09}$} & 0.42 $_{\pm0.01}$& 1.98$_{\pm0.02}$ & \tbrown{1.12$_{\pm0.01}$} &\tblue{3.97$_{\pm0.09}$}& \tblue{0.29$_{\pm0.00}$} & \tblue{4.67$_{\pm0.06}$}\\
    & ArtGS &\tbrown{0.74$_{\pm0.99}$} & \tblue{1.91$_{\pm0.07}$} & \tblue{0.23$_{\pm0.00}$} & 9.01$_{\pm0.23}$& 4.53$_{\pm1.59}$ &\tblue{1.21$_{\pm0.55}$} & 11.76$_{\pm0.51}$& \tbrown{7.43$_{\pm0.13}$} & 1.28$_{\pm0.29}$ & \tbrown{5.67$_{\pm0.15}$}\\
    & Ours-b & 0.34$_{\pm0.00}$ & 3.76$_{\pm0.12}$&F& \tbrown{8.32$_{\pm0.22}$} &\tblue{0.26$_{\pm0.05}$} &1.62$_{\pm0.13}$ & 1.13$_{\pm0.07}$& F & 1.54$_{\pm0.01}$ & 7.28 $_{\pm2.75}$ \\
    & Ours &0.38$_{\pm0.01}$&4.31$_{\pm0.10}$& 1.32$_{\pm0.12}$& 8.66$_{\pm0.44}$&\tbrown{0.26$_{\pm0.01}$} & \tbrown{1.30$_{\pm0.21}$} & \tblue{1.06$_{\pm0.07}$}& 9.44$_{\pm0.49}$&1.73$_{\pm0.01}$ & 5.86$_{\pm0.13}$\\
      \bottomrule
    \end{tabular}}
\end{table}
\begin{table}[t]
    \caption{\textbf{Quantitative evaluation on DTA-multi (with two moving parts) dataset}. We follow~\citep{weng2024neural,liu2025building} to obtain the metrics over 10 trials and report them as mean$\pm$std.
}
    \label{tab:comparison-to-soat}
    
    \resizebox{1\textwidth}{!}{ 
    \begin{tabular}{c|c|c|c|c|c|c|c|c|c|c|c}
    \toprule
    \multirow{2}*{}& \multirow{2}*{Method} &  \multicolumn{4}{c|}{Part-0}&  \multicolumn{4}{c|}{Part-1} &\multirow{2}*{CD-s} & \multirow{2}*{CD-w}\\
        \cmidrule{3-10}
      & &  Axis Ang&Axis Pose & Part Motion &CD-m&  Axis Ang&Axis Pose & Part Motion &CD-m& & \\
      \midrule
      \multirow{4}*{Fridge}& PARIS-m &21.27$_{\pm12.67}$ &2.30$_{\pm3.09}$&46.45$_{\pm11.63}$ &131.92$_{\pm48.64}$&73.26$_{\pm13.81}$&0.49$_{\pm0.40}$&166.29$_{\pm 14.79}$  &639.12$_{\pm54.42}$&5.17$_{\pm 0.95}$ &6.39$_{\pm 0.84}$\\
      & DTA & 1.55$_{\pm1.22}$ &\textbf{0.69$_{\pm1.05}$} & 14.33$_{\pm15.14}$ & 18.03$_{\pm6.02}$ &13.08$_{\pm3.23}$  & 94.98$_{\pm74.37}$ &  173.92$_{\pm8.77}$ & 220.55$_{\pm42.04}$ & 3.61$_{\pm0.53}$ & \textbf{2.03$_{\pm0.01}$}\\
      & ArtGS & 13.94$_{\pm9.59}$  &46.95$_{\pm12.83}$&176.52$_{\pm1.04}$&  11.80$_{\pm4.01}$ &3.33$_{\pm1.33}$&15.79$_{\pm6.24}$&41.81$_{\pm4.22}$& 11.24$_{\pm1.91}$ & \textbf{0.98$_{\pm0.19}$}&2.07$_{\pm0.21}$ \\
       & Ours & \textbf{0.68$_{\pm0.31}$} &3.58$_{\pm1.04}$& \textbf{3.57$_{\pm1.74}$}&\textbf{3.85$_{\pm1.61}$}& \textbf{1.67$_{\pm0.62}$}& \textbf{0.68$_{\pm0.47}$}&\textbf{ 4.81$_{\pm1.71}$} & \textbf{2.12$_{\pm1.39}$}& 8.16$_{\pm0.38}$ &5.40$_{\pm0.22}$ \\
        \midrule
     \multirow{4}*{Storage}& PARIS-m &F  &F&F &F&F&$-$&F  &F&F &F\\
      & DTA & 38.98$_{\pm 16.26}$  & 7.16$_{\pm2.24}$  &89.25$_{\pm2.39}$ &363.68$_{\pm102.26}$ & \textbf{0.24$_{\pm0.07}$} &$-$&\textbf{0.00$_{\pm0.00}$} & 221.74$_{\pm28.91}$ & \textbf{3.02$_{\pm0.14}$}  & \textbf{1.91$_{\pm0.03}$}\\
      & ArtGS &20.63$_{\pm6.83}$  &3.83$_{\pm2.03}$&107.56$_{\pm1.89}$ &252.69$_{\pm14.57}$&1.75$_{\pm1.50}$ &$-$&0.13$_{\pm0.12}$  &\textbf{1.26$_{\pm0.30}$}&3.76$_{\pm0.56}$ & 3.51$_{\pm0.40}$\\
       & Ours & \textbf{0.56$_{\pm0.77}$} & \textbf{1.26$_{\pm0.74}$} & \textbf{1.66$_{\pm1.04}$}& \textbf{0.81$_{\pm0.06}$} &1.03$_{\pm0.89}$& $-$& 0.06$_{\pm0.05}$& 27.35$_{\pm15.99}$& 10.37$_{\pm0.92}$ &6.87$_{\pm0.21}$\\
      \bottomrule
    \end{tabular}}
\end{table}

\begin{figure}[!t]
    \vspace{-10pt}
    \centering\includegraphics[width=0.95\linewidth]{ICLR 2025 Template/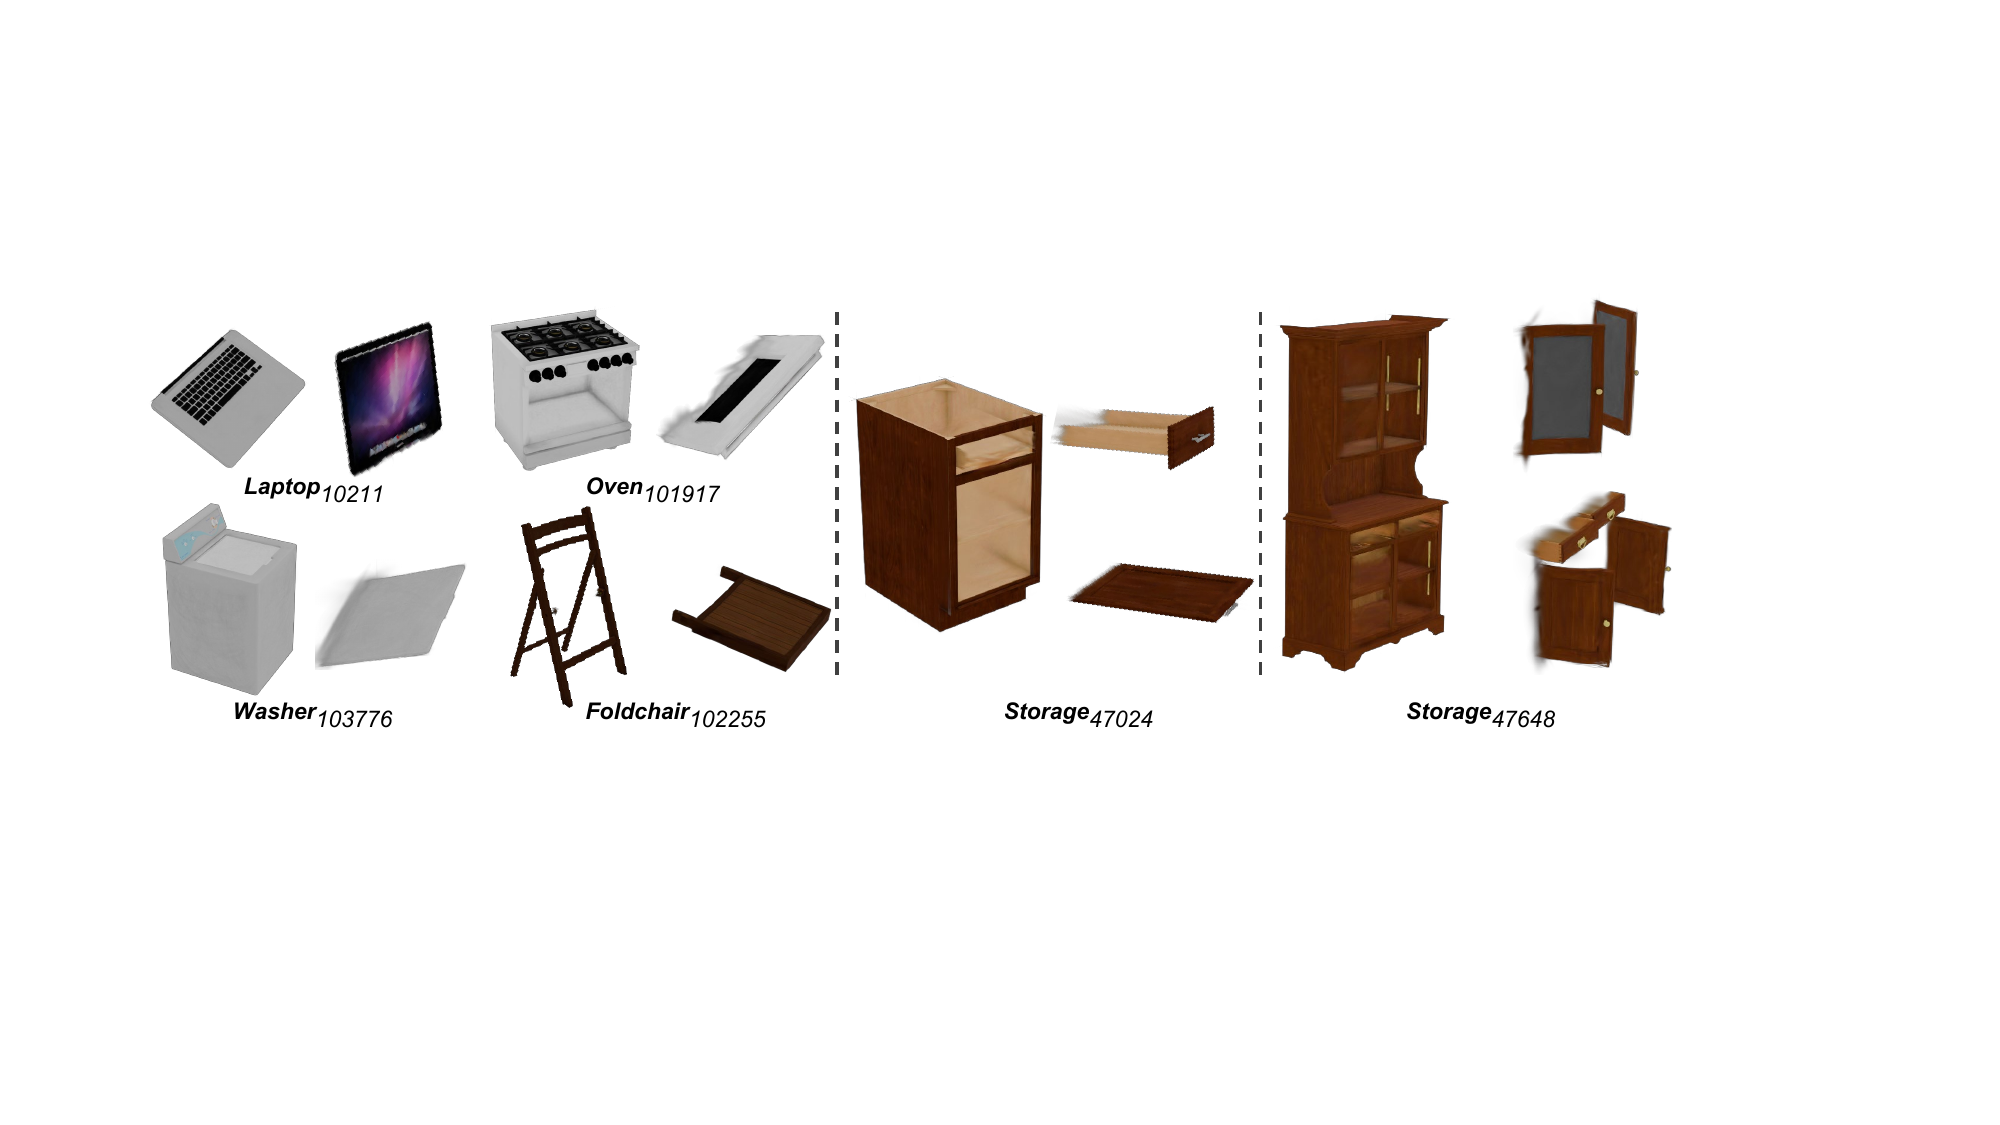}
    \vspace{-5pt}
    \caption{Rendering of our dual-Gaussian representation (\textbf{left}: static result $\{\mathcal{R}^{S}\}$, \textbf{right}: moving result $\{\mathcal{R}^{M, t\!=\!1}\}$). All objects (\textit{${\text{category}}_{\text{instance}}$}) are from PartNet-Mobility dataset~\citep{Mo_2019_CVPR}.}
    \label{fig:dualGS}
    \vspace{-10pt}
\end{figure}

\begin{figure}[!t]
 \vspace{-5pt}
    \centering\includegraphics[width=1\linewidth]{ICLR 2025 Template/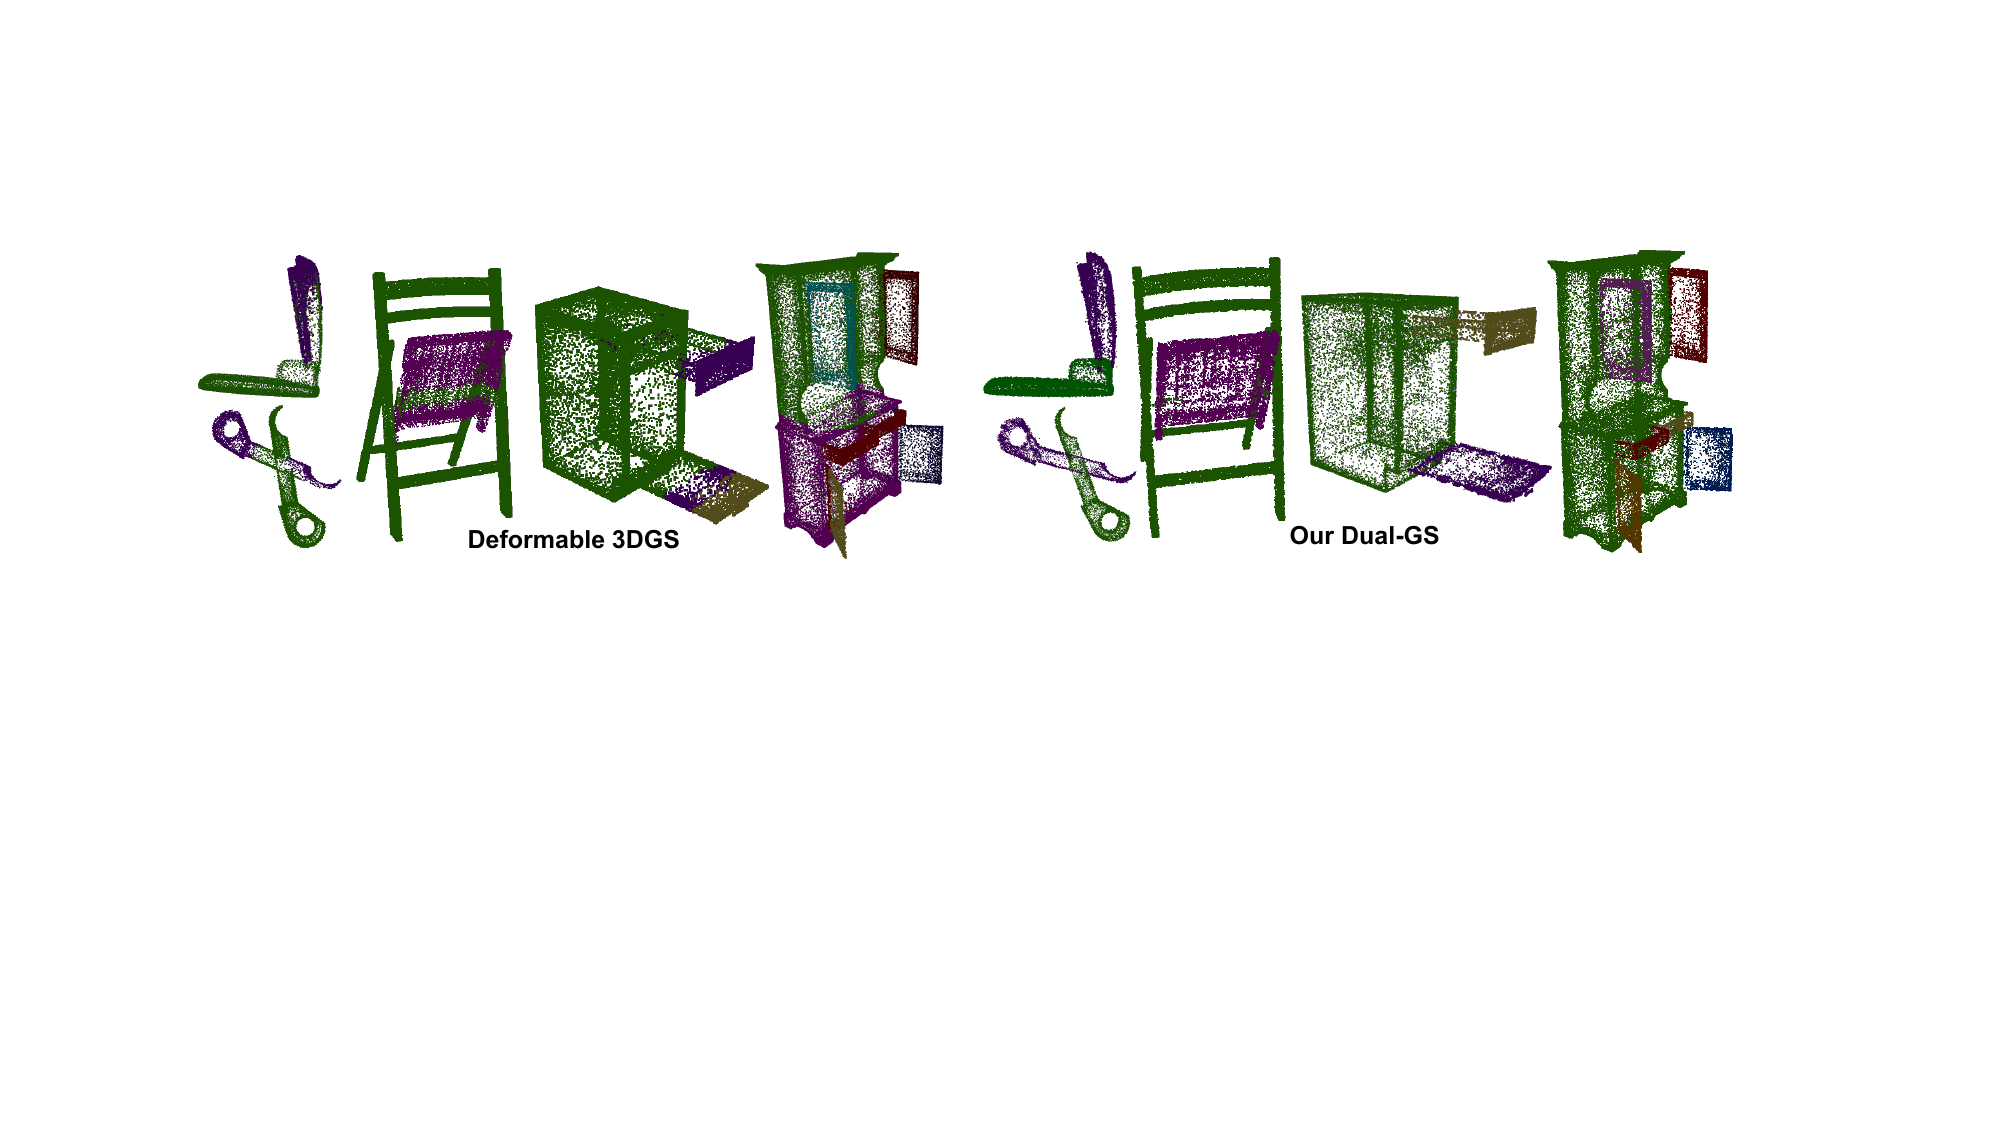}
    \caption{Part segmentation results based on Deformable 3DGS and our dual-Gaussian representation. We cluster Gaussians using the same sequential RANSAC settings; colours denote groups. Static noise in Deformable 3DGS noticeably degrades the segmentation.}
    \label{fig:compare_baseGS}
     \vspace{-10pt}
\end{figure}
